# Supplementary material for: Data-Driven Set-Based Estimation using Matrix Zonotopes with Set Containment Guarantees
Source: arXiv:2101.10784 source file (2022-03-27)
Supplement: Supplementary file 1 [file 9-appendix.tex]

%!TEX root = ../main.tex
\cleardoublepage
\section{Appendix (Temporary)} 
\label{sec:appendix}

\subsection{SVD method explanation}

\noindent We have a measurement equation 
\begin{align}
  y(k) = C x(k) + v(k), \;\;\; v(k) \in \mathcal{Z}_{v}(k),
  \label{eq:measurement}
\end{align}

The objective is to determine a set $\mathcal{Z}_{x|y}$ which 
  is the set of all possible $x \in \mathbb{R}^n$ which correspond to 
  \eqnref{eq:measurement} given $y \in \mathbb{R}^p$ and $\mathcal{Z}_{v}(k)$.\\

Let us consider the possibilities on the size and rank of $C$.
$C \in \mathbb{R}^{p \times n}$, $x \in \mathbb{R}^n$ and $\texttt{rank}(C) = r$.\\

\noindent If $C$ has rank condition $r < n$
\begin{enumerate}
  \item $r < n < p$ or $r < p < n$ or $r < p = n$\\
  In this case, the $svd(C)$ is as follows 
  \begin{align*}
    C = \begin{bmatrix}
      U_1 & U_2
    \end{bmatrix}
    \begin{bmatrix}
      \Sigma & 0 \\ 0 & 0
    \end{bmatrix}
    \begin{bmatrix}
      V_1^T \\ V_2^T
    \end{bmatrix}
  \end{align*}
  \item $r = p < n$ \\
  In this case, 
  \begin{align*}
    C = \begin{bmatrix}
      U_1
    \end{bmatrix}
    \begin{bmatrix}
      \Sigma & 0 
    \end{bmatrix}
    \begin{bmatrix}
      V_1^T  \\ V_2^T
    \end{bmatrix}
  \end{align*}
  which gives the same result as in the case $r < n < p$
\end{enumerate}
where the set corresponding to possible $x$ states is 
\begin{align*}
  \mathcal{Z}_{x|y} = \zono{V_1\Sigma^{-1}U_1^T(y-c_v), \; [V_1\Sigma^{-1}U_1^TG_v \; MV_2]}
\end{align*}
Note that we construct the generator matrix 
  with a mapping of $G_v$ to the range space of $C$, 
  as well as large, theoretically unbounded values in the 
  directions of the null space of $C$.
We need this because in the case that $r < n$, the measurement $y$ 
  does not contain enough information to fully bound the 
  possible values of $x$ satisfying the measurement equation.\\

\noindent If $C$ has rank condition $r = n$
\begin{enumerate}
  \item $r = n < p$ \\
  In this case, 
  \begin{align*}
    C = \begin{bmatrix}
      U_1 & U_2
    \end{bmatrix}
    \begin{bmatrix}
      \Sigma \\ 0 
    \end{bmatrix}
    \begin{bmatrix}
      V_1^T 
    \end{bmatrix}
  \end{align*}
  where the set $\mathcal{Z}_{x|y}$ becomes 
  \begin{align*}
    \mathcal{Z}_{x|y} = \zono{V_1\Sigma^{-1}U_1^T(y-c_v), \; V_1\Sigma^{-1}U_1^TG_v}
  \end{align*} 
  which is the same as using the pseudo-inverse of $C$, 
    i.e. $C^{\dagger} = V_1\Sigma^{-1}U_1^T$. The set $\mathcal{Z}_{x|y}$ is then 
    simplified as 
    \begin{align*}
      \mathcal{Z}_{x|y} = \zono{C^\dagger(y-c_v), \; C^\dagger G_v}
    \end{align*}
  \item $r = n = p$ \\
  In this case, $C$ is invertible, and can be written as 
  \begin{align*}
    C = U\Sigma  V^T \implies C^{-1} = V\Sigma^{-1}U^T
  \end{align*}
  and a direct solution 
    can be found as  
    \begin{align*}
      \mathcal{Z}_{x|y} = \zono{C^{-1}(y-c_v), \; C^{-1} G_v}
    \end{align*} 
\end{enumerate}

In the case that $r = n$, the set of $x$ that satisfies the measurement equation 
  will be bounded. 
Note that we no longer add a nullspace component $V_2$ in the 
  generator matrix since the nullspace of $C$ only contains the $0$ vector.

\noindent \textbf{Summary}\\

The result is that we can always use the SVD of $C$, 
  with appropriately portioned submatrices $U,\Sigma,V$.
By determining $r$ w.r.t $n$, we can either add the nullspace component $V_2$
  to the generator or not.
This means that the method is general, 
  and applicable to any form of $C$.\\

\newpage
\subsection{Re-writing the proof}

\begin{proposition}
  Given a measurement $y^i(k)$ with noise  
    $v^i(k) \in \mathcal{Z}_{v,i} = \zono{c_{v,i},G_{v,i}}$ 
    satisfying \eqnref{eq:observations},
  the possible states $x$ that correspond to this measurement,
    assuming $\|x\|_2 \leq K \in \mathbb{R}_{\geq 0}$,  
  are contained within the zonotope
  $ \mathcal{Z}_{x|y^i} = \zono{c_{x|y^i},G_{x|y^i}},$
  where
  \begin{equation}
    \begin{split}
      c_{x|y^i} &= V_1 \Sigma^{-1}U_1^T\big( y^i(k) - c_{v,i} \big), \\
      G_{x|y^i} &= \begin{bmatrix} 
        V_1 \Sigma^{-1}U_1^T G_{v,i} & V_2 M
    \end{bmatrix},
    \end{split}
    \label{eq:prop_1_eqn}
  \end{equation} 
  for all $M \geq K$, with $U_1$, $V_1$, $\Sigma$ and $V_2$ 
    obtained from the SVD of $C^i$.
  Assuming $C^i$ has rank $r^i$, then 
  \begin{align}
    C^i = \begin{bmatrix}
        U_1 & U_2
      \end{bmatrix}
      \begin{bmatrix}
        \Sigma_{r^i \times r^i} & 0_{r^i \times (n-r^i)} \\ 
        0_{(p^i-r^i)\times r^i} & 0_{(p^i-r^i)\times(n-r^i)}
      \end{bmatrix}
      \begin{bmatrix}
        V_1^\top \\ V_2^\top
      \end{bmatrix}.
      \label{eq:svd_of_C}
  \end{align}
  \label{prop:measurement_zonotope}
\end{proposition}
\begin{proof}
  From \eqnref{eq:svd_of_C}, 
    we rewrite \eqnref{eq:observations} 
    as $U_1\Sigma V_1^\top x = y^i - v^i$,
    so $x = V_1\Sigma^{-1}U_1^\top (y^i - v^i)$.
  Since $v^i$ is bounded by $\mathcal{Z}_{v,i}$,
  % letting $x \in \zono{c_{x|y^i},G_{x|y^i}}$, 
  we can write  
    \begin{align*}
      x= \underbrace{V_1 \Sigma^{-1}U_1^T\big( y^i - c_{v,i}\big)}_{c_{x|y^i}} - 
        \underbrace{V_1 \Sigma^{-1}U_1^T G_{v,i}}_{G_{x|y^i}'} \beta, \;\; |\beta| \leq 1.
    \end{align*}
  This set corresponds to all possible $x$ values 
    within the range space of $C^i$ satisfying \eqnref{eq:observations}.
  By definition, if $r^i = n$, then $V_2 = \emptyset$, 
    $V_1$ spans the domain of $x$,
    and $\zono{c_{x|y^i},G_{x|y^i}'}$ sufficiently defines all possible $x$
    satisfying \eqnref{eq:observations}.
  However, 
    if $r^i < n$, $V_1$ only spans a subset of the domain of $x$.
  To ensure $\mathcal{Z}_{x|y^i}$ contains all possible $x$
    we need to include a basis for $\texttt{ker}(C^i)$ in $G_{x|y^i}$.
  This is done by appending the generator $V_2M$ to $G_{x|y^i}$,
  and ensuring $M \geq K$ such that $V_2M$ includes all $x$ values in $V_2$
    such that $\|x\|_2 \leq K$. 
  In both cases for $r^i$, the generator matrix can be written as
  \begin{align*}
    G_{x|y^i} 
    = \begin{bmatrix} 
      G_{x|y^i}' & V_2M 
    \end{bmatrix} 
    = \begin{bmatrix} 
      V_1 \Sigma^{-1}U_1^T G_{v,i} & V_2M 
    \end{bmatrix}, 
  \end{align*}
  and the set $\mathcal{Z}_{x|y^i} = \zono{c_{x|y^i}, G_{x|y^i}}$.
  This result extends to the case when $r^i < p^i$ using 
   similar argumentation in the respective cases $r^i = n$ and $r^i < n$. 
\end{proof}

\begin{remark}
  In our use-case, the set $\mathcal{Z}_{x|y^i(k)}$ will be 
    intersected with $\Rpredict$ at each time step.
  It is therefore sufficient to set $M > \texttt{radius}(\Rpredict_k) + \|V_2^\top c_k\|_2$
    instead of the more conservativate $M > K$.
  $c_k$ is the center of $\Rpredict_k$, and 
    $\texttt{radius}(\Rpredict_k)$ 
    returns the radius of a minimal hypersphere containing $\Rpredict_k$
    \cite{conf:cora}.
\end{remark}

\newpage
\subsection{Previous iteration of M bound in remark}

\begin{proposition}
  Given a measurement $y^i(k)$ and  
    $v^i(k) \in \mathcal{Z}_{v,i} = \zono{c_{v,i},G_{v,i}}$ 
    satisfying \eqnref{eq:observations},
  the possible states $x$ that correspond to this measurement 
  are contained within the zonotope
  $ \mathcal{Z}_{x|y^i} = \zono{c_{x|y^i},G_{x|y^i}},$
  where
  \begin{equation}
    \begin{split}
    c_{x|y^i} &= V_1 \Sigma^{-1}U_1^T\big( y^i(k) - c_v \big), \\
    G_{x|y^i} &= \begin{bmatrix} 
      V_1 \Sigma^{-1}U_1^T G_v & V_2 M
    \end{bmatrix},
  \end{split}
  \label{eq:prop_1_eqn}
  \end{equation} 
  where $U_1$, $V_1$, $\Sigma$ and $V_2$ are obtained from the SVD of $C^i$ as
  \begin{align}
    C^i =  
    \begin{bmatrix}
        U_1 & U_2
      \end{bmatrix}
      \begin{bmatrix}
        \Sigma & 0 \\ 0 & 0
      \end{bmatrix}
      \begin{bmatrix}
        V_1^T \\ V_2^T
      \end{bmatrix}
      \label{eq:svd_of_C}
  \end{align}
  and $M \gg 0$ (theoretically, $M \to \infty$).
  \label{prop:measurement_zonotope}
\end{proposition}
\begin{proof}
  Consider the SVD of $C^i$ in \eqnref{eq:svd_of_C}.
  By definition, $C^i$ has rank 
    $r^i = \texttt{rank}(C^i) \leq \min(p^i,n)$.
  We omit the $(k)$'s for clarity. By computing the singular value decomposition of $C^i$, we can rewrite \eqref{eq:observations} as 
   \begin{align*}
   U_1 \Sigma V_1^T x  = y^i - v^i \implies  x=V_1 \Sigma^{-1}U_1^T\big( y^i - v^i \big),
  \end{align*} 
  since $U_1$ and $V_1$ are orthogonal. 
  Recall that $v^i$ is unknown, but bounded by $\mathcal{Z}_{v,i}$. 
  Let $x \in \zono{c_{x|y^i},G_{x|y^i}}$. Then we obtain
  \begin{align*}
    x= \underbrace{V_1 \Sigma^{-1}U_1^T\big( y^i - c_{v,i}\big)}_{c_{x|y^i}} - 
      \underbrace{V_1 \Sigma^{-1}U_1^T G_{v,i}}_{G_{x|y^i}'} \beta .
  \end{align*}
   Finally, since the null-space of $C^i$ contains all values of $x$ not 
    observable from the mapping $C^i$, we need $\mathcal{Z}_{x|y^i}$ to contain 
    these. If $r^i < n$, $V_2 \neq \emptyset$ spans $\texttt{ker}(C^i)$. 
  To ensure $\mathcal{Z}_{x|y^i}$ contains the unobservable states,
     we include the generators $V_2M$ where $M \to \infty$.
   $G_{x|y^i}$ can be computed as follows
  \begin{align*}
  G_{x|y^i} 
  = \begin{bmatrix} G_{x|y^i}' & V_2M \end{bmatrix} 
  = \begin{bmatrix} V_1 \Sigma^{-1}U_1^T G_{v,i} & V_2M \end{bmatrix}. 
  \end{align*} 
\end{proof}
\begin{remark}
  The requirement that $M \to \infty$ in \propref{prop:measurement_zonotope}  
  is not implementable in practice,
    since zonotopes must remain bounded.
  However, since we will find the intersection of $\mathcal{Z}_{x|y^i}(k)$ 
    with $\Rpredict_k$, we can choose any $M$ as long as 
    $ M > \text{radius} \big( V_2^\top \Rpredict_k \big) + || V_2^\top c_k ||_F $ 
    where $c_k$ is the center of $\Rpredict_k$.
\end{remark}
